# Supplementary material for: Hopfions in lattice dimer model
Source: arXiv:1901.04527 source file (2019-06-12)
Supplement: Supplementary file 1 [file SupplementalMaterial_3_Fig_10_2.pdf]

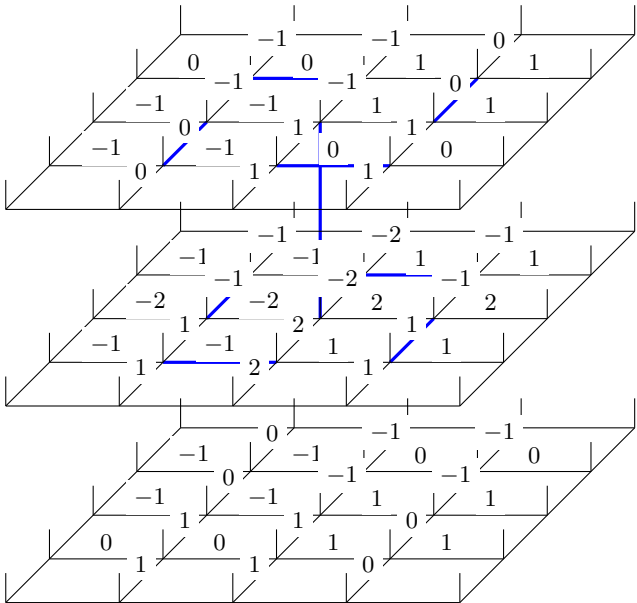

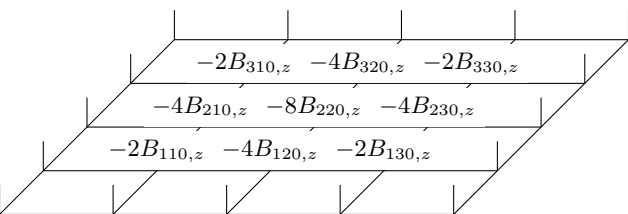

(a)

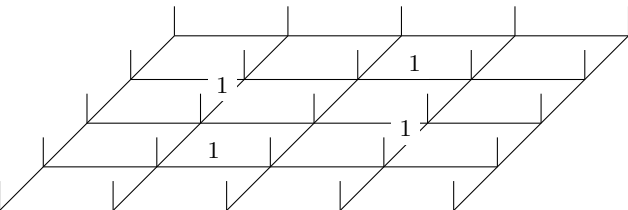

(b)
