# Supplementary material for: Hopfions in lattice dimer model
Source: arXiv:1901.04527 source file (2019-06-12)

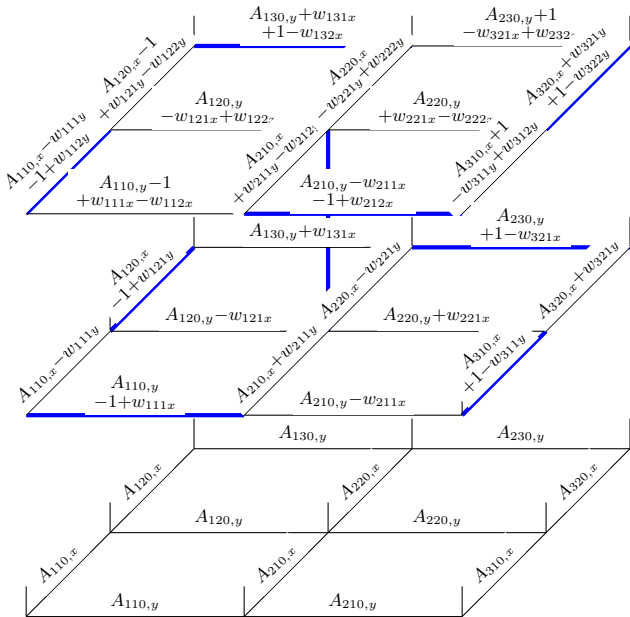

Supplement: Supplementary file 3 [file SupplementalMaterial_3_Fig_9_2.pdf]
